# Supplementary material for: MAGELLAN: Metacognitive predictions of learning progress guide autotelic LLM agents in large goal spaces
Source: arXiv:2502.07709 source file (2025-06-17)
Supplement: Supplementary file 1 [file Appendix_A.tex]

<In this section we present additional information about the environment: first an example of textual input for the LLM-based RL agent \ref{app:zoo_ex_obs} and second a table containing detailed information for each goal category \ref{app:details_goal_categories}.  
\subsection{Example of observation}
\label{app:zoo_ex_obs}

\begin{figure}[htbp]
\centering
\begin{tcolorbox}[myboxstyle]
Goal: Grow blue elephant\\
You see: baby blue elephant, baby green grizzly, red pea seed, blue water\\
You are on: baby blue elephant\\
Inventory (2/2): red carrot, green potato
\end{tcolorbox}
\caption{\textbf{An observation in the Playground-Text-Zoo environment.} In this state, the agent is standing on a baby blue elephant and can use the plants in its inventory to make it grow by performing the action \texttt{"Release all"}.}
\label{fig:playground_obs}
\end{figure}

\subsection{Details over each goals categories} \label{app:details_goal_categories}

The goals are grouped by categories that share the same strategy and which can be inferred from the semantic of the goals. For instance \textit{Grow cow} and \textit{Grow deer} are part of \textit{Grow big herbivore}. We fix the maximal number of actions to be $50\%$ longer than the optimal strategy. Table~\ref{tab:optimal_trajectories_categories} contains more details on each category.

\begin{table}[!ht]
\caption{The optimal trajectories per categories.}
\label{tab:optimal_trajectories_categories}
\begin{tabular}{|c|c|c|c|}
\hline
\multirow{2}{*}{Categories}           & \multirow{2}{*}{Optimal action strategy}              & Minimal number & Maximal number \\
                     &                                          & of actions     & of actions     \\ \hline
Grasp X              & Go to X, Grasp                           & 2              & 3              \\ \hline
\multirow{2}{*}{Grow plant} & Go to water, Grasp, Go to plant, & \multirow{2}{*}{4}              & \multirow{2}{*}{6}              \\
                     & Release water &              &             \\ \hline
\multirow{2}{*}{Grow small herbivore} & Go to water, Grasp, Go to plant, & \multirow{2}{*}{7}              & \multirow{2}{*}{11}              \\
                     & Release water, Grasp, Go to herbivore, release plant &              &             \\ \hline
\multirow{3}{*}{Grow small carnivore} & Go to water, Grasp, Go to plant, & \multirow{3}{*}{10}              & \multirow{3}{*}{15}              \\
                     & Release water, Grasp, Go to herbivore, release plant, &              &             \\
                     & Grasp, Go to carnivore, release &              &             \\ \hline
\multirow{4}{*}{Grow big herbivore} & Go to water, Grasp, Go to plant, & \multirow{4}{*}{12}              & \multirow{4}{*}{18}              \\
                     & Release water, Grasp, Go to water, Grasp &              &             \\ 
                     & Go to plan, Release water, Grasp, Go to herbivore, &              &             \\ 
                     & Release all &              &             \\ \hline
\multirow{4}{*}{Grow big carnivore} & Go to water, Grasp, Go to plant, & \multirow{4}{*}{15}              & \multirow{4}{*}{23}              \\
                     & Release water, Grasp, Go to water, Grasp &              &             \\ 
                     & Go to plan, Release water, Grasp, Go to herbivore, &              &             \\ 
                     & Release all, Grasp, Go to carnivore, Release herbivore &              &             \\ \hline
\end{tabular}
\end{table}
