# Supplementary material for: MAGELLAN: Metacognitive predictions of learning progress guide autotelic LLM agents in large goal spaces
Source: arXiv:2502.07709 source file (2025-06-17)
Supplement: Supplementary file 2 [file Appendix_B.tex]

\label{app:implementation_details}
\subsection{LLM-based RL agent}\label{app:sac_glam}
We use a discrete Soft Actor-Critic \cite{Christodoulou2019SoftAF} adaptation of PPO-GLAM \cite{carta_grounding_2023}.
We first follow PPO-GLAM's approach to obtaining the policy using an LLM by computing the probability of each action $ a_i \in \mathcal{A} $ as the probability of its token sequence $ a_i = \{ w_1, w_2, ..., w_{|a_i|} \} $ (with $w_i \in \mathcal{V} $) to follow a prompt $p$ containing both $o$ and $g$.
Then, we add a two hidden layers (1024 units with ReLU) Multi-Layer Perceptron (MLP) on top of the last hidden state from the decoder to obtain the critic, similarly to how PPO-GLAM learns the value function.

However, SAC requires computing the Q-value for all possible actions given a state. To compute them, we use an MLP with a single output and give both the observation-goal pair and an action as input to the LLM. While this requires as many forward passes as the number of possible actions, this best exploits the representation produced by the LLM. See Figure~\ref{fig:sac_glam} for a schema of the RL agent's architecture. We provide in Table~\ref{tab:sac_param} the hyperparameters we used.

\begin{figure}[!ht]
    \centering
    \includegraphics[width=0.5\linewidth]{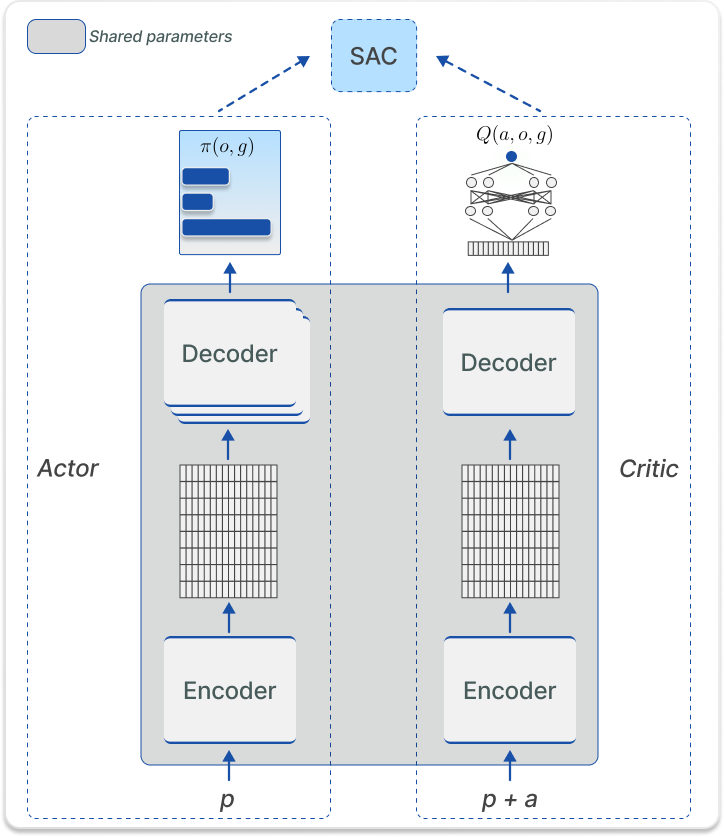}
    \caption{Our LLM-based RL agent using a SAC adaptation of GLAM.}
    \label{fig:sac_glam}
\end{figure}

\begin{table}[!ht]
    \caption{SAC hyperparameters}
    \centering 
    \begin{tabular}{ll}
    \hline
    \textbf{Variable} & \textbf{Value} \\
    \hline
    Update frequency & $64$ \\
    Number of updates & $1$ \\
    Batch size & $256$ \\
    Discount factor & $0.99$ \\
    Optimizer & Adam \\
    Critic learning rate & $1 \times 10^{-4}$ \\
    Actor learning rate & $1 \times 10^{-4}$ \\
    Entropy coefficient & auto \\
    Entropy coefficient initialization & $0.05$ \\
    Target entropy & $0.0005$ \\
    Entropy coefficient learning rate & $2 \times 10^{-3}$ \\
    n-step & $3$ \\
    Replay buffer capacity & $100000$ \\
    \hline
    \end{tabular}
    \label{tab:sac_param}
\end{table}

\subsection{MAGELLAN}\label{app:magellan}

\subsection{Moving average LP estimator}\label{app:lp_estimator}
We follow the Model Babbling method from \cite{Forestier2016ModularAC} to estimate the LP of each goal.
We keep a per-goal history of the last $N$ success rates. Every time this goal $g$ is sampled, a new ALP measure $\hat{ALP}(g)$ is obtained by computing the average of the absolute difference between the new goal' binary reward and every reward from the history. This goal's ALP (and utility in the Multi-Armed Bandit) is updated with a moving average between the current utility and the new ALP measure:
\[
ALP(g) = \alpha ALP(g) + (1-\alpha) \hat{ALP}(g)
\]

In our experiments, we use $N=100$ and $\alpha=0.3$.

\subsection{Compute budget}
To optimize GPU VRAM usage during training, we employed LoRA \citep{Hu2021LoRALA} and 4-bit quantization techniques as described in \citep{Dettmers2023QLoRAEF}.

We used a vectorized version of Little-Zoo with 32 instances of the environment running (synchronously) in parallel. In order to accelerate the use of an LLM as the trained RL policy (and critic), we leveraged Lamorel\footnote{https://github.com/flowersteam/lamorel} as in GLAM and deployed 4 instances of the LLM in parallel (distributing both the forward passes to compute the actions' probability and the training in a Data Parallelism setting).
When using Flan-T5 250M, each LLM instance is distributed (Vertical Model Parallelism) over one Nvidia V100 32GB GPUs requiring thus a total of 4 Nvidia V100 32GB GPUs to run an experiment (1 GPU $\times$ 4 LLM instances). In total, each experiment and ablation requires 80 GPU hours per seed on the Nvidia V100 32GB.
