# Supplementary material for: MAGELLAN: Metacognitive predictions of learning progress guide autotelic LLM agents in large goal spaces
Source: arXiv:2502.07709 source file (2025-06-17)
Supplement: Supplementary file 3 [file Appendix_C.tex]

\subsection{\textbf{Q1} \& \textbf{Q2}} \label{app:additional_results_q1q2}

In this section we plot the success rate for each goal categories for MALP and MAGELLAN per seed. We 

\subsubsection{MALP results over training}
\label{app:additional_results_q1q2_MALP}
We report in figures~\ref{fig:app_q1q2_classic_seed0}, ~\ref{fig:app_q1q2_classic_seed1}, ~\ref{fig:app_q1q2_classic_seed2} and ~\ref{fig:app_q1q2_classic_seed3} the per-seed and per-category SR over training goals. We also plot the arms' utility (i.e. estimated LP).

We also report the per-seed evolution of sampled goals from each category in Figure~\ref{fig:app_q1q2_malp_sampling}.

\begin{figure}[!ht]
    \centering
    \includegraphics[width=0.8\linewidth]{Figures/Q1_2/appendix/classic_train_seed_0.png}
    \caption{Per-category SR and utility (i.e. estimated LP) on training goals for seed 0.}
    \label{fig:app_q1q2_classic_seed0}
\end{figure}

\begin{figure}[!ht]
    \centering
    \includegraphics[width=0.8\linewidth]{Figures/Q1_2/appendix/classic_train_seed_1.png}
    \caption{Per-category SR and utility (i.e. estimated LP) on training goals for seed 1.}
    \label{fig:app_q1q2_classic_seed1}
\end{figure}

\begin{figure}[!ht]
    \centering
    \includegraphics[width=0.8\linewidth]{Figures/Q1_2/appendix/classic_train_seed_2.png}
    \caption{Per-category SR and utility (i.e. estimated LP) on training goals for seed 2.}
    \label{fig:app_q1q2_classic_seed2}
\end{figure}

\begin{figure}[!ht]
    \centering
    \includegraphics[width=0.8\linewidth]{Figures/Q1_2/appendix/classic_train_seed_3.png}
    \caption{Per-category SR and utility (i.e. estimated LP) on training goals for seed 3.}
    \label{fig:app_q1q2_classic_seed3}
\end{figure}

\begin{figure}[!ht]
    \centering
    \includegraphics[width=0.8\linewidth]{Figures/Q1_2/appendix/malp_sampling_proportion_train.png}
    \caption{Per-seed sampling proportion when using MALP.}
    \label{fig:app_q1q2_malp_sampling}
\end{figure}

\subsubsection{MAGELAN results over training}
\label{app:additional_results_q1q2_MAGELLAN}
We report in figures~\ref{fig:app_q1q2_magellan_seed0}, ~\ref{fig:app_q1q2_magellan_seed1}, ~\ref{fig:app_q1q2_magellan_seed2} and ~\ref{fig:app_q1q2_magellan_seed3} the per-seed and per-category SR over training goals. We also plot the estimated SR and LP. The estimated SR and delayed estimated SR follow closely the true SR even when it drops suddenly. Moreover the small inertia in the prediction tends to help smoothing the LP prediction (especially if you compare to MALP Appendix~\ref{app:additional_results_q1q2_MALP}) avoiding abrupt transition in the sampling.

We also report the per-seed evolution of sampled goals from each category in Figure~\ref{fig:app_q1q2_magellan_sampling}.

\begin{figure}[!ht]
    \centering
    \includegraphics[width=0.8\linewidth]{Figures/Q1_2/appendix/magellan_train_seed_0.png}
    \caption{Per-category SR along with MAGELLAN's estimation of SR and LP on training goals for seed 0.}
    \label{fig:app_q1q2_magellan_seed0}
\end{figure}

\begin{figure}[!ht]
    \centering
    \includegraphics[width=0.8\linewidth]{Figures/Q1_2/appendix/magellan_train_seed_1.png}
    \caption{Per-category SR along with MAGELLAN's estimation of SR and LP on training goals for seed 1.}
    \label{fig:app_q1q2_magellan_seed1}
\end{figure}

\begin{figure}[!ht]
    \centering
    \includegraphics[width=0.8\linewidth]{Figures/Q1_2/appendix/magellan_train_seed_2.png}
    \caption{Per-category SR along with MAGELLAN's estimation of SR and LP on training goals for seed 2.}
    \label{fig:app_q1q2_magellan_seed2}
\end{figure}

\begin{figure}[!ht]
    \centering
    \includegraphics[width=0.8\linewidth]{Figures/Q1_2/appendix/magellan_train_seed_3.png}
    \caption{Per-category SR along with MAGELLAN's estimation of SR and LP on training goals for seed 3.}
    \label{fig:app_q1q2_magellan_seed3}
\end{figure}

\begin{figure}[!ht]
    \centering
    \includegraphics[width=0.8\linewidth]{Figures/Q1_2/appendix/magellan_sampling_proportion_train.png}
    \caption{Per-seed sampling proportion when using MAGELLAN.}
    \label{fig:app_q1q2_magellan_sampling}
\end{figure}

\subsection{\textbf{Q3}} \label{app:additional_results_q3}

\subsection{\textbf{Q4}} \label{app:additional_results_q4}

In Figure~\ref{fig:app_q4_sr} we plot the success rate per-seed and per-category for MAGELAN and MALP. It appears that MAGELLAN helps the agent to better maintain its performances on goals it already mastered (see seed 1 on \textit{grow small herbivore}). MAGELLAN by preventing the uniform sampling just after the transition allow the agent to discover faster more difficult categories (see seed 2 and 3 on \textit{grow small herbivore}).
\begin{figure}[!ht]
    \centering
    \includegraphics[width=0.8\linewidth]{Figures/Q4/appendix/per_seed_adaptation.png}
    \caption{Per-seed and per-category evolution of SR when switching from training to test goals when training the policy with MAGELLAN and MALP.}
    \label{fig:app_q4_sr}
\end{figure}
